# Supplementary material for: A Framework for Learning Assessment through Multimodal Analysis of Reading Behaviour and Language Comprehension
Source: arXiv:2110.11938 source file (2021-10-22)
Supplement: Supplementary file 1 [file Experiment_Questions-Only_Brain-teasing_puzzles.pdf]

## Day-1, Session-1 Puzzle

**Questions:**

**1.1) How many squares are there in the following figure ?**

**Ans:**

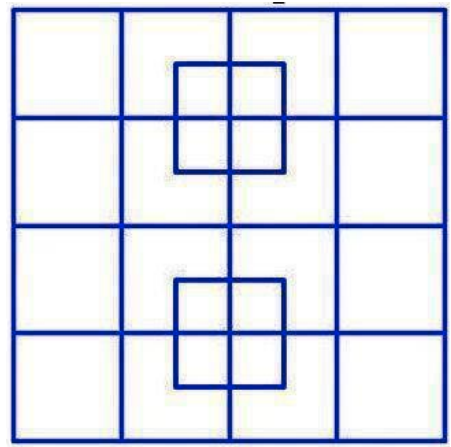

**1.2) Which number comes next? 1 3 8 13 21 ?**

**Ans:**

**1.3) Which number replaces the question marks?**

**Ans:**

Which number replaces the question mark?

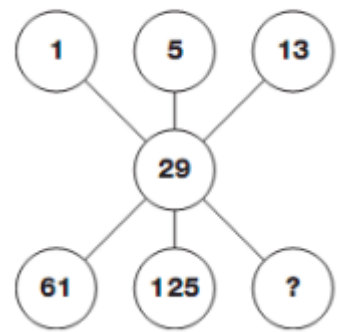

**1.4) Four friends built a colony for themselves. They built their own houses at different distances from each other.**

**C lived 60 km away from A. D lived 40 km away from B. C lived 10 km nearer to D than he lived to B. Can you find out how far was D's house from A?**

**Ans:**

## Day-1, Session-2 Puzzle

**Questions:**

**2.1) Which number should replace the question mark In The Circle Below ?**

**Ans:**

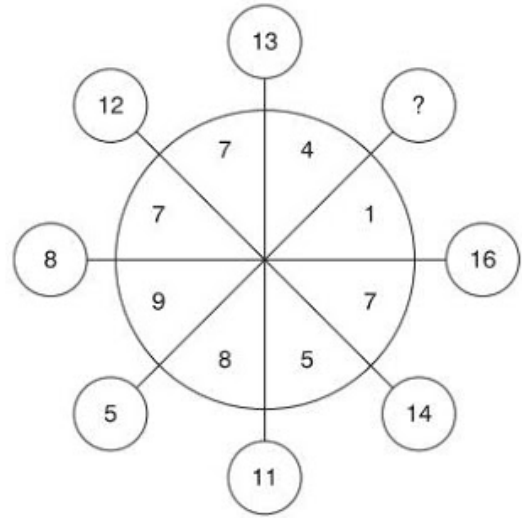

**2.2) Can you count the number of minutes in Feb 2017?**

**Ans:**

**2.3) I spend \$50 in the way below. Where is my missing \$1**

**Ans:**

| Spend     | Balance   |
|-----------|-----------|
| 20        | 30        |
| 15        | 15        |
| 9         | 6         |
| 6         | 0         |
| <b>50</b> | <b>51</b> |

**2.4) Which number replaces the question mark?**

**Ans:**

| 10 |    |
|----|----|
| 8  | 13 |
| 16 | 6  |
| 4  | 19 |
| 22 | ?  |

## Day-2, Session-1 Puzzle

Questions:

3.1) Count the triangles in picture below.

Ans:

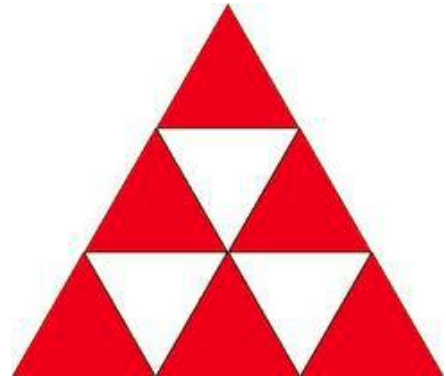

3.2) In the picture below, can you identify the value of angle 'Y'?

Ans:

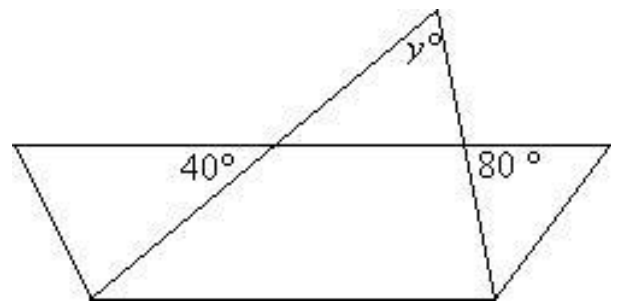

3.3) Which number will come next in the series? 2 4 3 9 4 6 1 5 5 2 6 6 3 7 ?

Ans:

3.4) We have black but we are not tea seeds. We have white but we are not lime. We have water but we are not a river. We have feather but we are not birds. Who are we?

Ans:

3.5) There are 5 sisters in the room: Ann is reading a book, Margaret is cooking, Kate is playing chess, Marie is doing laundry. What is the fifth sister doing?

Ans:

3.6) How these possible:

- 2 + 2 = fish
- 3 + 3 = eight
- 7 + 7 = triangle

Ans:

## Day-2, Session-2 Puzzle

**Questions:**

**4.1) Can you replace the "?" mark with the correct number ?**

**Ans:**

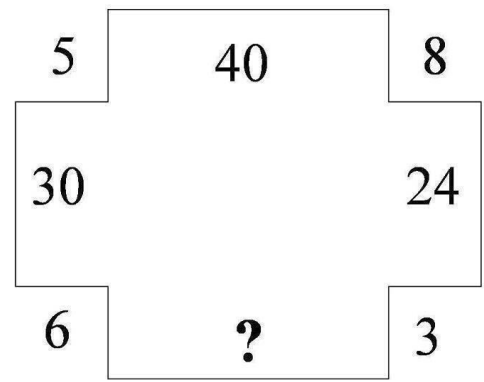

**4.2) Which number will replace the "?" in the picture below?**

**Ans:**

|   |   |    |
|---|---|----|
| 3 | 1 | 7  |
| 6 | 4 | 34 |
| 8 | 7 | 71 |
| 9 | 8 | ?  |

**4.3) Can you list words which sound alike with the different meaning? One means the "state of rest" while the other word is related to "writing material".**

**Ans:**

**4.4) There is a common word pattern in the below words. Can you find it?**

1. CHARM
2. DYNAMO
3. YAM
4. REAY
5. EAR
6. TOADY

**Ans:**

### Day-3, Session-1 Puzzle

**Questions:**

**5.1) Which shape will follow next?**

**Ans:**

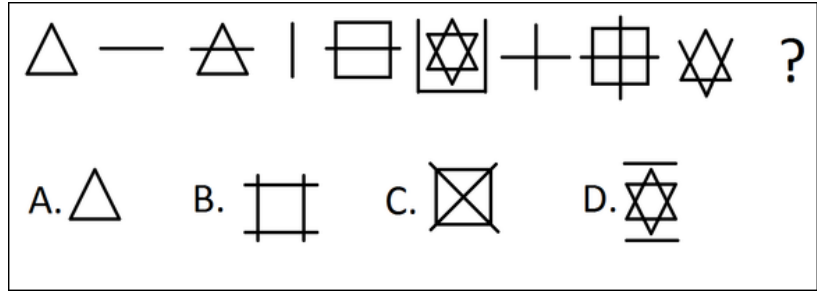

**5.2) What number comes inside the circle?**

**Ans:**

What number comes inside the circle?

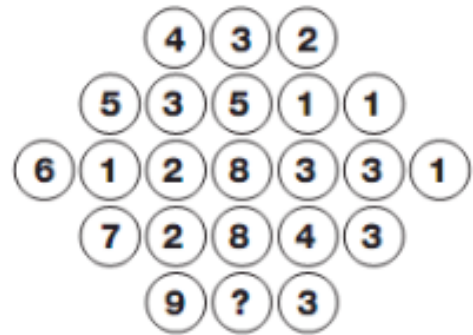

**5.3) I am the end of life but also the start of earth.**

**I wait in the middle of the ocean but not there in the bank.**

**I stay very close to the beginning of the death.**

**I am able to enter in the heaven but also there in the midst of the hell.**

**What Am I?**

**Ans:**

**5.4) Can you name a three letter English verb that becomes its past tense simple by moving first letter at the end?**

**Ans:**

**5.5) I have keys without key locks. I have space without rooms. You can enter but you cannot go outside. What am I?**

**Ans:**

**5.6) When I'm first said, I'm quite mysterious. But when I'm explained, I'm nothing serious.**

**What am I?**

**Ans:**

### Day-3, Session-2 Puzzle

**Questions:**

**6.1) Which number replaces the question marks?**

**Ans:**

Which number replaces the question mark?

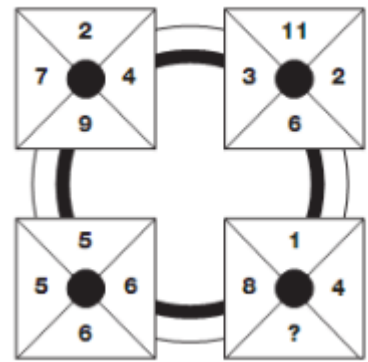

**6.2) Consider,**

A = 1

B = 2

C = 3

...

...

Z = 26.

**Based on above code, Find the famous 11 letter word whose digit is equal to 51.**

**Ans:**

**6.3) What does this message say ?**

**G T Y O R J O T E O U I A B G T**

*Hint*

*Count the letters and try splitting the letters up into groups.*

**Ans:**

**6.4) I have six faces and twenty-one eyes, yet I can not see. What am I?**

**Ans:**
