# Supplementary material for: A Framework for Learning Assessment through Multimodal Analysis of Reading Behaviour and Language Comprehension
Source: arXiv:2110.11938 source file (2021-10-22)
Supplement: Supplementary file 2 [file questionnaire.pdf]

Participant's Id:

Age:

Gender:

Course and Semester:

Enrollment No:

Eyeglass During Experiment: Yes / No

Mother Tongue:

Experiment Date:

**Set 1: Please fill up the blank with suitable word:**

- a) The Camel lived in the middle of a \_\_\_\_\_ Desert.
- b) Horse came to the Camel on \_\_\_\_\_ morning.
- c) The Camel ate \_\_\_\_\_ and \_\_\_\_\_ and \_\_\_\_\_.
- d) When anybody spoke to the Camel, he said \_\_\_\_\_ Just \_\_\_\_\_ and no more.
- e) The Camel missed \_\_\_\_\_ days, which were: \_\_\_\_\_, \_\_\_\_\_, \_\_\_\_\_.

**Set 2: Please choose a perfect option from multiple choices:**

- a) *And the Camel went away to join the Three. And from that day to this the Camel always wears a hump (we call it 'hump' now, not to hurt his feelings); but he has never yet caught up with the three days that he missed at the beginning of the world, and he has never yet learned how to behave.*

The word “**behave**” in the passage is closest in meaning to

- i) act, ii) live, iii) learn, iv) say, v) I DON'T KNOW
- b) The Ox came to The Camel, with the yoke on his neck on \_\_\_\_\_.  
i) Monday, ii) Tuesday, iii) Wednesday, iv) Thursday, v) I DON'T KNOW
- c) Djinn was \_\_\_\_\_ of All Deserts.  
i) king, ii) in charge, iii) owner, iv) worker, v) I DON'T KNOW
- d) Select mismatched word in following options  
i) plough, ii) prickle, iii) trot, iv) fetch and carry, v) I DON'T KNOW.
- e) The Camel looked at his \_\_\_\_\_ in the pool of water.  
i) own reflection, ii) owner's face reflection, iii) friends' reflection, iv) owner's dust-cloak, v) I DON'T KNOW.

\*\*\*\*\*

Participant's Id:

Age:

Gender:

Course and Semester:

Enrollment No:

Eyeglass During Experiment: Yes / No

Mother Tongue:

Experiment Date:

**Set 1: Please fill up the blank with suitable word:**

- The Camel lived in the middle of a \_\_\_\_\_ Desert.
- Dog came to the Camel with a \_\_\_\_\_.
- The Camel ate \_\_\_\_\_ and \_\_\_\_\_ and \_\_\_\_\_.
- When anybody spoke to the Camel, he said \_\_\_\_\_ Just \_\_\_\_\_ and no more.
- The Camel missed \_\_\_\_\_ days, which were: \_\_\_\_\_, \_\_\_\_\_, \_\_\_\_\_.

**Set 2: Please choose a perfect option from multiple choices:**

- And the Camel went away to join the Three. And from that day to this the Camel always wears a hump (we call it 'hump' now, not to hurt his feelings); but he has never yet caught up with the three days that he missed at the beginning of the world, and he has never yet learned how to **behave**.*

The word "**behave**" in the passage is closest in meaning to

- act, ii) live, iii) learn, iv) say, v) I DON'T KNOW
- Presently the Horse came to him on \_\_\_\_\_ morning, with a saddle on his back.  
i) Monday, ii) Tuesday, iii) Wednesday, iv) Thursday, v) I DON'T KNOW
  - That made the Three very angry, and they held a \_\_\_\_\_ on the edge of the Desert.  
i) meeting, ii) senate, iii) visit, iv) panchayat, v) I DON'T KNOW
  - Select mismatched word in following options  
i) plough, ii) prickle, iii) trot, iv) fetch and carry, v) I DON'T KNOW.
  - The Djinn rolled himself up in his \_\_\_\_\_, and took a walk across the Desert, and found the Camel looking at his own reflection in a pool of water.  
i) own reflection, ii) desert, iii) chin in his hand, iv) dust-cloak, v) I DON'T KNOW.

\*\*\*\*\*

Participant's Id:

Age:

Gender:

Course and Semester:

Enrollment No:

Eyeglass During Experiment: Yes / No

Mother Tongue:

Experiment Date:

**Set 1: Please fill up the blank with suitable word:**

- a) The Camel lived in the middle of a \_\_\_\_\_ Desert.
- b) Horse came to the Camel on \_\_\_\_\_ morning.
- c) The Camel ate \_\_\_\_\_ and \_\_\_\_\_ and \_\_\_\_\_.
- d) When anybody spoke to the Camel, he said \_\_\_\_\_ Just \_\_\_\_\_ and no more.
- e) The Camel missed \_\_\_\_\_ days, which were: \_\_\_\_\_, \_\_\_\_\_, \_\_\_\_\_.

**Set 2: Please choose a perfect option from multiple choices:**

- a) *And the Camel went away to join the Three. And from that day to this the Camel always wears a hump (we call it 'hump' now, not to hurt his feelings); but he has never yet caught up with the three days that he missed at the beginning of the world, and he has never yet learned how to behave.*

The word "**behave**" in the passage is closest in meaning to

- i) act, ii) live, iii) learn, iv) say, v) I DON'T KNOW
- b) Presently the Ox came to him, with \_\_\_\_\_  
i) a yoke on his back ii) a saddle on his neck, iii) a saddle on his back, iv) the yoke on his neck  
v) I DON'T KNOW
- c) That made the Three very angry, and they held a \_\_\_\_\_ on the edge of the Desert.  
i) meeting, ii) senate, iii) visit, iv) panchayat, v) I DON'T KNOW
- d) Select mismatched word in following options  
i) account of your idleness, ii) wait a minute, iii) Certainly not, iv) Djinn of All Deserts,  
v) I DON'T KNOW.
- e) Presently there came along the Djinn who was in charge of All Deserts \_\_\_\_\_  
i) in the pool of water, ii) desert, iii) rolling in a cloud of dust, iv) dust-cloak, v) I DON'T  
KNOW.

\*\*\*\*\*

Participant's Id:

Age:

Gender:

Course and Semester:

Enrollment No:

Eyeglass During Experiment: Yes / No

Mother Tongue:

Experiment Date:

Set 1: Please fill up the blank with suitable word:

- a) During his administration \_\_\_\_\_ immeasurably enlarged the power of the presidency.
- b) \_\_\_\_\_ held different attitudes toward the changes brought about by the market, banks, and commerce.
- c) The Whigs, in contrast, viewed government power \_\_\_\_\_.
- d) \_\_\_\_\_ attracted farmers isolated from the market or uncomfortable with it.
- e) This “\_\_\_\_\_” of bankers and investors manipulated the banking system for their own profit.

Set 2: Please choose a perfect option from multiple choices:

- a) *During his administration he **immeasurably** enlarged the power of the presidency. “The President is the direct representative of the American people,” he lectured the Senate when it opposed him.*

The word “immeasurably” in the passage is closest in meaning to

A. frequently B. greatly C. rapidly D. reportedly E. I DON'T KNOW

- b) *The author mentions bankers and investors in the passage as an example of which of the following?*

A. The Democratic Party's main source of support  
B. The people that Democrats claimed were unfairly becoming rich  
C. The people most interested in a return to a simple agrarian republic  
D. One of the groups in favor of Andrew Jackson's presidency  
E. I DON'T KNOW

- c) The development of the modern presidency in the United States began with Andrew Jackson who swept to power in \_\_\_\_\_ at the head of the Democratic Party and served until \_\_\_\_\_.

A. 1829 B. 1830 C. 1836 D. 1837 E. DON'T KNOW

- d) Select mismatched word in following options

A. Votes B. farmers C. society D. history E. I DON'T KNOW

- e) The Whigs were supported by which of the following groups:

A. workers unhappy with the new industrial system B. planters involved in international trade  
C. rising entrepreneurs D. individuals seeking to open the economy to newcomers  
E. I DON'T KNOW.

\*\*\*\*\*

Participant's Id:

Age:

Gender:

Course and Semester:

Enrollment No:

Eyeglass During Experiment: Yes / No

Mother Tongue:

Experiment Date:

Set 1: Please fill up the blank with suitable word:

- a) During his administration \_\_\_\_\_ immeasurably enlarged the power of the presidency.
- b) \_\_\_\_\_ held different attitudes toward the changes brought about by the market, banks, and commerce.
- c) The Whigs, in contrast, viewed government power \_\_\_\_\_.
- d) \_\_\_\_\_ attracted farmers isolated from the market or uncomfortable with it.
- e) This “\_\_\_\_\_” of bankers and investors manipulated the banking system for their own profit.

Set 2: Please choose a perfect option from multiple choices:

- a) The presidency of Andrew Jackson was especially significant for which of the following reasons?
  - A. The President granted a portion of his power to the Senate.
  - B. The President began to address the Senate on a regular basis.
  - C. It was the beginning of the modern presidency in the United States.
  - D. It was the first time that the Senate had been known to oppose the President.
  - E. I DON'T KNOW
- b) Whigs and Democrats differed not only in their attitudes toward the market but also about how active the central government should be in people's lives. Despite Andrew Jackson's **inclination** to be a strong President, Democrats as a rule believed in limited government. Government's role in the economy was to promote competition by destroying monopolies and special privileges.

The word **inclination** in the passage is closest in meaning to

- A. argument    B. tendency    C. example    D. warning    E. I DON'T KNOW
- c) The development of the modern presidency in the United States began with Andrew Jackson who swept to power in \_\_\_\_\_ at the head of the Democratic Party and served until \_\_\_\_\_.
  - A. 1829      B. 1830      C. 1836      D. 1837      E. 1838      F. DON'T KNOW
- d) Select mismatched word in following options
  - A. planters    B. businesspeople    C. bankers    D. newcomers    E. I DON'T KNOW
- e) The Democrats were supported by all of the following groups EXCEPT
  - A. workers unhappy with the new industrial system    B. planters involved in international trade
  - C. rising entrepreneurs    D. individuals seeking to open the economy to newcomers
  - E. I DON'T KNOW

\*\*\*\*\*

Participant's Id:

Age:

Gender:

Course and Semester:

Enrollment No:

Eyeglass During Experiment: Yes / No

Mother Tongue:

Experiment Date:

**Set 1: Please fill up the blank with suitable word:**

- a) During his administration \_\_\_\_\_ immeasurably enlarged the power of the presidency.
- b) \_\_\_\_\_ held different attitudes toward the changes brought about by the market, banks, and commerce.
- c) The Whigs, in contrast, viewed government power \_\_\_\_\_.
- d) \_\_\_\_\_ attracted farmers isolated from the market or uncomfortable with it.
- e) This “\_\_\_\_\_” of bankers and investors manipulated the banking system for their own profit.

**Set 2: Please choose a perfect option from multiple choices:**

- a) The presidency of Andrew Jackson was especially significant for which of the following reasons?
  - A. The President granted a portion of his power to the Senate.
  - B. The President began to address the Senate on a regular basis.
  - C. It was the beginning of the modern presidency in the United States.
  - D. It was the first time that the Senate had been known to oppose the President.
  - E. I DON'T KNOW
- b) Which of the following can be inferred about variations in political beliefs within the Whig Party?
  - A. They were focused on issues of public liberty.
  - B. They caused so members to leave the Whig party.
  - C. They were unimportant to most Whigs.
  - D. They reflected regional interests.
- c) The development of the modern presidency in the United States began with Andrew Jackson who swept to power in \_\_\_\_\_ at the head of the Democratic Party and served until \_\_\_\_\_.
  - A. 1829      B. 1830      C. 1836      D. 1837      E. 1838      F. DON'T KNOW
- d) According to the article, a Democrat would be most likely to support government action in which of the following areas?
  - A. Creating a state religion      B. Supporting humanitarian legislation
  - C. Destroying monopolies      D. Recommending particular moral beliefs
- e) Complete the summary by selecting the **THREE** answer choices that express the most important ideas in the passage. Some answer choices do not belong in the summary because they express ideas that are not presented in the passage or are minor ideas in the passage.

**The political system of the United States in the mid-nineteenth century was strongly influenced by the social and economic circumstances of the time.**

- A. The Democratic and Whig Parties developed in response to the needs of competing economic and political constituencies.
- B. During Andrew Jackson's two terms as President, he served as leader of both the Democratic and Whig Parties.
- C. The Democratic Party primarily represented the interests of the market, banks, and commerce.
- D. In contrast to the Democrats, the Whigs favored government aid for education.
- E. A fundamental difference between Whigs and Democrats involved the importance of the market in society.
- F. The role of government in the lives of the people was an important political distinction between the two parties.

\*\*\*\*\*
